# Supplementary material for: Bias Reduction via Cooperative Bargaining in Synthetic Graph Dataset Generation
Source: arXiv:2205.13901 source file (2022-05-27)
Supplement: Supplementary file 1 [file 7_appendix.tex]

\newpage

\begin{appendices}

\section{Validation dataset description}

\input{tables/validation}

\end{appendices}
